# Supplementary material for: Bubble breakup probability in turbulent flows
Source: arXiv:2403.08684 source file (2025-05-08)
Supplement: Supplementary file 1 [file SupplementaryMaterialRiviere2024.pdf]

# Supplementary Material to Bubble breakup probability in turbulent flows

Aliénor Rivière<sup>1\*</sup> and Stéphane Perrard<sup>1</sup>

<sup>1</sup>*PMMH, CNRS, ESPCI Paris, Université PSL, Sorbonne Université, Université de Paris, 75005, Paris, France*

(Dated: March 13, 2024)

In this Supplementary Material, we explain how to generate a realisation of  $\mathcal{T}(t)$ , the effective forcing from turbulence on bubble shape, using Gaussssian copula.

## CONTENTS

|                                                                   |   |
|-------------------------------------------------------------------|---|
| I. Principle and notations                                        | 1 |
| A. Constructing $\mathcal{T}$ from a vector of Gaussian variables | 1 |
| B. Explicit expression of each function                           | 2 |
| II. Determination of the Covariance matrix $\Sigma'$              | 3 |
| A. Diagonal terms                                                 | 3 |
| B. Off-Diagonal terms                                             | 3 |
| C. Conclusion                                                     | 4 |
| III. Verification                                                 | 4 |

## I. PRINCIPLE AND NOTATIONS

### A. Constructing $\mathcal{T}$ from a vector of Gaussian variables

Let  $\mathcal{T}$  be the forcing evolution that we want to evaluate and  $\{\mathcal{T}_i\}_{i \in [1, N]}$  its discrete counterpart, defined at times  $\{t_i\}_{i \in [1, N]}$ . We assume the statistics of  $\mathcal{T}$  to be stationary, so that all  $\mathcal{T}_i$  share the same distribution and the covariance matrix of  $\{\mathcal{T}_i\}_{i \in [1, N]}$  is such that  $\text{Cov}(\mathcal{T}_i, \mathcal{T}_j)$  only depends on  $|t_i - t_j|$ . We introduce the following notations:

- $\Phi_{\sigma_{\mathcal{T}}}$ : probability density function of  $\mathcal{T}$
- $\sigma_{\mathcal{T}}$ : standard deviation of  $\mathcal{T}$
- $A(t)$ : autocorrelation function of  $\mathcal{T}$
- $Y_i = \mathcal{T}_i / \sigma_{\mathcal{T}}$
- $\Sigma$ : covariance matrix of  $\{Y_i\}_{i \in [1, N]}$ .

By definition of  $\{Y_i\}_{i \in [1, N]}$ , we have the following properties:

- $Y_i$  has distribution  $\Phi_1$ , denoted  $\Phi$  in what follows
- $\Sigma_{i,j} = A(|t_i - t_j|)$
- $\Sigma_{ii} = 1$ , ie the standard deviation of  $Y_i$  is 1 for all i.

Finally, we introduce  $F_{\Phi}$  the cumulative distribution of  $\Phi$  and  $F_{\Phi}^{-1}$  its inverse.

There is no method to directly compute  $\{Y_i\}_{i \in [1, N]}$ . Instead, we will construct  $\{Y_i\}_{i \in [1, N]}$  using a vector of centered gaussian variables  $\{X_i\}_{i \in [1, N]}$ : this is a gaussian copula method. Since we aim at constructing a stationary process, all the  $X_i$  also share the same normal distribution  $\mathcal{N}$  with average 0 and standard deviation  $\sigma'$ . We introduce these additional notations:

---

\* [alienor.riviere@espci.fr](mailto:alienor.riviere@espci.fr)

- $\Sigma'$ : covariance matrix of  $\{X_i\}_{i \in [1, N]}$
- $F_{\mathcal{N}}$ : cumulative distribution function of  $\mathcal{N}$
- $F_{\mathcal{N}}^{-1}$ : inverse cumulative distribution function of  $\mathcal{N}$

We can easily generate a Gaussian random vector  $\{X_i\}_{i \in [1, N]}$  of any covariance matrix  $\Sigma'$ . The idea is then to transform  $\{X_i\}_{i \in [1, N]}$  into  $\{Y_i\}_{i \in [1, N]}$ . We know that we can construct  $Z_i$  of distribution  $\Phi$  through

$$Z_i = F_{\Phi}^{-1}(F_{\mathcal{N}}(X_i)).$$

However, the covariant matrix of  $\{Z_i\}_{i \in [1, N]}$  is not known a priori. As a consequence, the difficulty is to find the right  $\Sigma'$  so that after applying  $F_{\Phi}^{-1}(F_{\mathcal{N}}(\cdot))$  to each  $X_i$ , we get a vector with covariance matrix  $\Sigma$ . In what follows we will determine  $\Sigma'$  and then deduce  $Y_i$  using,

$$Y_i = F_{\Phi}^{-1}(F_{\mathcal{N}}(X_i)). \quad (1)$$

The following expression will also be useful:

$$X_i = F_{\mathcal{N}}^{-1}(F_{\Phi}(Y_i)). \quad (2)$$

### B. Explicit expression of each function

The distribution  $\Phi$  is the hyperbolic secant distribution with standard deviation 1:

$$\Phi(x) = \frac{1}{2} \frac{1}{\cosh\left(\frac{\pi x}{2}\right)}$$

Its associated cumulative distribution function is,

$$F_{\Phi} = \frac{2}{\pi} \arctan\left(\exp\left(\frac{\pi x}{2}\right)\right),$$

whose inverse is

$$F_{\Phi}^{-1} = \frac{2}{\pi} \log\left(\tan\left(\frac{\pi x}{2}\right)\right).$$

The centered normal distribution,  $\mathcal{N}$  is

$$\mathcal{N}(x) = \frac{1}{\sigma' \sqrt{2\pi}} \exp\left[-\frac{1}{2} \left(\frac{x}{\sigma'}\right)^2\right].$$

Its cumulative distribution function is,

$$F_{\mathcal{N}}(x) = \frac{1}{2} \left[1 + \operatorname{erf}\left(-\frac{x}{\sqrt{2}\sigma'}\right)\right]$$

whose inverse writes

$$F_{\mathcal{N}}^{-1}(x) = \sigma' \sqrt{2} \operatorname{erf}^{-1}[2x - 1].$$

We also introduce the joint law of two centered Gaussian variable  $X_i, X_j$  such that  $\operatorname{Var}(X_i) = \operatorname{Var}(X_j) = \Sigma'_{ii} = (\sigma')^2$  and  $\operatorname{Cov}(X_i, X_j) = \operatorname{Cov}(X_j, X_i) = \Sigma'_{ij}$ :

$$f_{ij}(x, y) = \frac{1}{2\pi \sqrt{\Delta_{ij}}} \exp\left(-\frac{\Sigma'_{ii}(x^2 + y^2) - 2\Sigma'_{ij}xy}{2\sqrt{\Delta_{ij}}}\right) \quad (3)$$

where  $\Delta_{ij} = (\Sigma'_{ii})^2 - (\Sigma'_{ij})^2$ .

Finally, the autocorrelation function of the forcing is,

$$A(t) = \exp\left(-2\pi \cdot 2^{2/3} t\right) (1 + 2\pi \cdot 2^{2/3} t)$$

## II. DETERMINATION OF THE COVARIANCE MATRIX $\Sigma'$

### A. Diagonal terms

We can explicitly compute  $\Sigma'_{ii}$  from  $\Sigma_{ii}$  using equation (2):

$$\begin{aligned}\Sigma'_{ii} &= \text{Var}(X_i) = (\sigma')^2 \\ &= \text{Var}(F_{\mathcal{N}}^{-1}(F_{\Phi}(Y_i))) \\ &= \int_{\mathbb{R}} F_{\mathcal{N}}^{-1}(F_{\Phi}(y))^2 \Phi(y) \mathbf{d}y - \left[ \int_{\mathbb{R}} F_{\mathcal{N}}^{-1}(F_{\Phi}(y)) \Phi(y) \mathbf{d}y \right]^2 \\ &= I_1(\Sigma_{ii}) - (I_2(\Sigma_{ii}))^2\end{aligned}$$

We estimate numerically these two integral and find  $I_1 = 1$  and  $I_2 = 0$  (indeed the integrand of  $I_2$  is odd). It follows,

$$\Sigma'_{ii} = (\sigma')^2 = \Sigma_{ii} = 1, \quad \forall i \quad (4)$$

### B. Off-Diagonal terms

This time, we want to evaluate  $\Sigma'_{ij}$  with  $i \neq j$ . We do not know the joint law of  $(Y_i, Y_j)$ , which is too costly to be evaluated, but we have an expression for the joint law of two Gaussian variables (equation (3)). We then use equation (1) to express  $\Sigma_{ij}$  as a function of  $\Sigma'_{ij}$ :

$$\begin{aligned}\Sigma_{i,j} &= \text{Cov}(Y_i, Y_j) \\ &= \text{Cov}[F_{\Phi}^{-1}(F_{\mathcal{N}}(X_i)), F_{\Phi}^{-1}(F_{\mathcal{N}}(X_j))] \\ &= \iint_{\mathbb{R}^2} F_{\Phi}^{-1}(F_{\mathcal{N}}(x_1)) F_{\Phi}^{-1}(F_{\mathcal{N}}(x_2)) f_{ij}(x_1, x_2) \mathbf{d}x_1 \mathbf{d}x_2 - \left[ \int_{\mathbb{R}} F_{\Phi}^{-1}(F_{\mathcal{N}}(x)) \mathcal{N}(x) \mathbf{d}x \right]^2 \\ &= I_a(\Sigma'_{ij}) + I_b^2\end{aligned}$$

Numerically, we find  $I_b = 0$  (the integrand is odd).

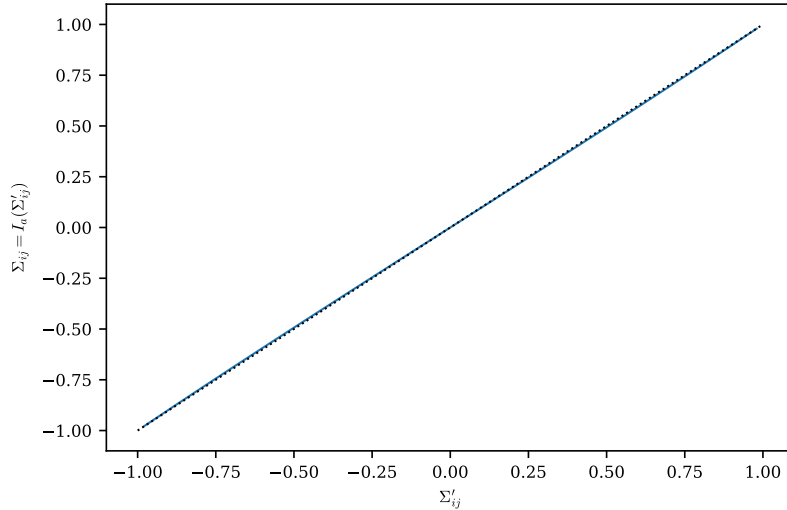

FIG. 1. Variation of  $\Sigma_{ij}$  with  $\Sigma'_{ij}$ . The blue line is  $I_a$ . The black dotted line follows  $\Sigma_{ij} = \Sigma'_{ij}$ .

We estimate  $I_a$  numerically (see figure 1) and find that  $I_a(\Sigma'_{ij}) = \Sigma'_{ij}$  is an excellent approximation. It follows that:

$$\Sigma_{ij} = \Sigma'_{ij}, \quad \forall i \neq j \quad (5)$$

### C. Conclusion

Combining equations (4) and (5) we have

$$\Sigma = \Sigma' \quad (6)$$

making the evaluation of  $\Sigma'$  in our case extremely fast and cheap.

### III. VERIFICATION

To summarize, we first generate a Gaussian random vector  $\{X_i\}_{i \in [1, N]}$  with covariant matrix,

$$\Sigma'_{ij} = A(|t_i - t_j|). \quad (7)$$

Then we use equation (1) to get  $\{Y_i\}_{i \in [1, N]}$ . Finally,  $\mathcal{T}_i$  is obtained using

$$\mathcal{T}_i = \sigma_{\mathcal{T}} Y_i. \quad (8)$$

Figures 2 and 3 compare the autocorrelation function and the distribution of  $\mathcal{T}_i$ , respectively, obtained with the above procedure, to their theoretical expressions. The agreement is excellent.

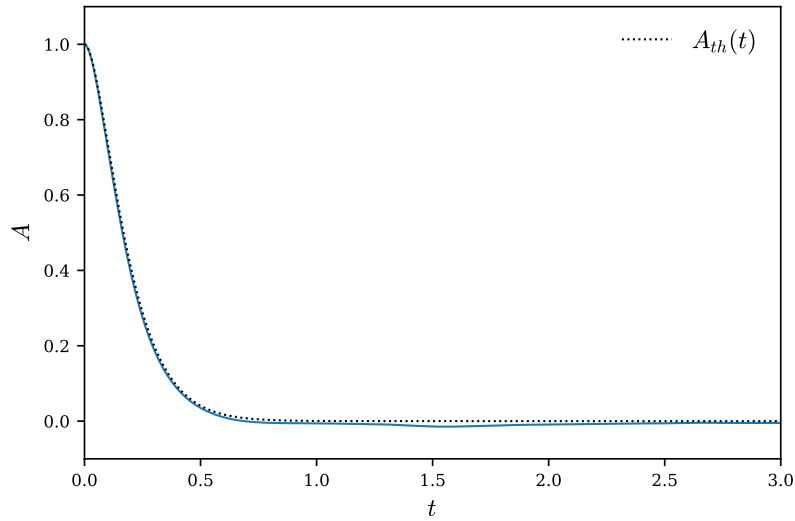

FIG. 2. Autocorrelation of  $\mathcal{T}_i$ , ie  $\Sigma'_{ij}$  as a function of time. The black dotted line is the targeted function. The blue line corresponds to the generated forcing signal.

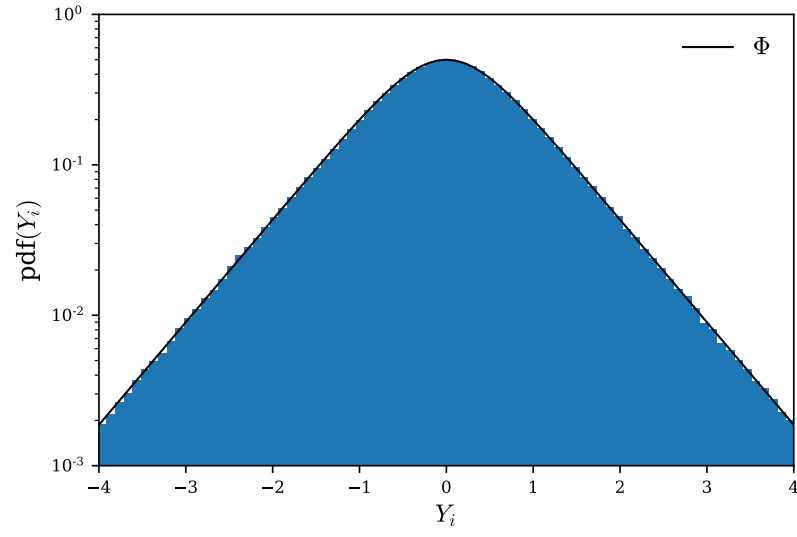

FIG. 3. Comparison between the distribution of the generated noise (in blue) and the theoretical target distribution (in black). The agreement is excellent.
